# Supplementary material for: Dynamical mean-field theory of the Anderson-Hubbard model with local and non-local disorder in tensor formulation
Source: arXiv:2105.06971 ancillary file (2021-05-14)
Supplement: Supplementary file 1 [file supplementary.pdf]

# Supplementary material
# Dynamical mean-field theory of the Anderson–Hubbard model with local and non-local disorder in tensor formulation


A. Weh,[1,*] Y. Zhang,[2] A. Östlin,[3,4] H. Terletska,[5] D. Bauernfeind,[6]
K.-M. Tam,[7,8] H. G. Evertz,[9] K. Byczuk,[10] D. Vollhardt,[3] and L. Chioncel[3,4]

[1] *Theoretical Physics II, Institute of Physics, University of Augsburg, 86135 Augsburg, Germany*
[2] *Kavli Institute of Theoretical Sciences, University of Chinese Academy of Sciences, Beijing, 100190, China*
[3] *Theoretical Physics III, Center for Electronic Correlations and Magnetism, Institute of Physics, University of Augsburg, 86135 Augsburg, Germany*
[4] *Augsburg Center for Innovative Technologies, University of Augsburg, 86135 Augsburg, Germany*
[5] *Department of Physics and Astronomy, Middle Tennessee State University, Murfreesboro, TN 37132, USA*
[6] *Center for Computational Quantum Physics, Flatiron Institute, 162 5th Avenue, New York, NY 10010, USA*
[7] *Department of Physics & Astronomy, Louisiana State University, Baton Rouge, LA 70803, USA*
[8] *Center for Computation & Technology, Louisiana State University, Baton Rouge, LA 70803, USA*
[9] *Institute of Theoretical and Computational Physics, Graz University of Technology, 8010 Graz, Austria*
[10] *Institute of Theoretical Physics, Faculty of Physics, University of Warsaw, ul. Pasteura 5, 02-093 Warszawa, Poland*



(Dated: May 14, 2021)


## I. NUMERICAL DATA AND SCRIPTS FOR FIGURES

The numerical data of the DMFT calculations for Figs. 2 to 5 is available in Ref. 1. The datasets are in the '`DMFT_data`' directory, see Table I for the specific directory names. The subdirectory '`lattice_output`' contains averaged local lattice Green's functions; the subdirectory '`imp_output`' contains the quantities of the effective impurity models calculated by the FTPS solver[2]. Besides the conditionally averaged local Green's functions $\mathbb{E}(G_{ii}(\omega)|i \mapsto \alpha)$, the HDF5 datasets contain additional information, like the BEB effective medium $\underline{\mathbf{S}}(\omega)$, the DMFT self-energy $\Sigma^{\alpha}(\omega)$, and the hybridization function $\Delta^{\alpha}(\omega)$ and its discretization.

Ref. 1 contains also the scripts to generate the plots Figs. 2 to 5 from the data. These scripts require our BEB implementation provided in Ref. 3.


* andreas.weh@physik.uni-augsburg.de



1 A. Weh, "Supplementary material: Dynamical mean-field theory of the Anderson–Hubbard model with local and non-local disorder in tensor formulation," Zenodo `https://doi.org/10.5281/zenodo.4762163` (2021).
2 D. Bauernfeind, M. Zingl, R. Triebl, M. Aichhorn, and H. G. Evertz, Phys. Rev. X **7**, 031013 (2017).
3 A. Weh and A. Östlin, "Derweh/gftools: Gftool 0.9.0 release," Zenodo `http://doi.org/10.5281/zenodo.4744546` (2021).

Table I. File directories giving the data shown in the Figures.

| Figure | parameter | directory |
|---|---|---|
| **2** | $\underline{\mathrm{T}}^{\mathsf{AB}} = 0$ | ‘U3V0c0.1_tab0’ |
| | $\underline{\mathrm{T}}^{\mathsf{AB}} = 0.5$ | ‘U3V0c0.1_tab0.5’ |
| | $\underline{\mathrm{T}}^{\mathsf{AB}} = 1.5$ | ‘U3V0c0.1_tab1.5’ |
| | $\underline{\mathrm{T}}^{\mathsf{AB}} = 5.0$ | ‘U3V0c0.1_tab5.0’ |
| not shown | $\underline{\mathrm{T}}^{\mathsf{AB}} = 1.7$ | ‘U3V0c0.1_tab1.7’ |
| **3** | $\underline{\mathrm{T}}^{\mathsf{AB}} = 0$ | ‘UaUb3V0c0.1_tab0’ |
| | $\underline{\mathrm{T}}^{\mathsf{AB}} = 0.5$ | ‘UaUb3V0c0.1_tab0.5’ |
| | $\underline{\mathrm{T}}^{\mathsf{AB}} = 1.5$ | ‘UaUb3V0c0.1_tab1.5’ |
| | $\underline{\mathrm{T}}^{\mathsf{AB}} = 5.0$ | ‘UaUb3V0c0.1_tab5’ |
| **4** | $\underline{\mathrm{U}}^{\mathsf{A}} = \underline{\mathbf{U}}^{\mathsf{B}} = 3D$ | |
| | $c^{\mathsf{A}} = 0.1$ | ‘U3V0c0.1_tab5’ |
| | $c^{\mathsf{A}} = 0.2$ | ‘U3V0c0.2_tab5.0’ |
| | $c^{\mathsf{A}} = 0.3$ | ‘U3V0c0.3_tab5.0’ |
| | $c^{\mathsf{A}} = 0.4$ | ‘U3V0c0.4_tab5.0’ |
| | $c^{\mathsf{A}} = 0.5$ | ‘U3V0c0.5_tab5.0’ |
| | $\underline{\mathrm{U}}^{\mathsf{A}} = 0, \underline{\mathbf{U}}^{\mathsf{B}} = 3D$ | |
| | $c^{\mathsf{A}} = 0.1$ | ‘Ua0Ub3V0c0.1_tab5’ |
| | $c^{\mathsf{A}} = 0.2$ | ‘Ua0Ub3V0c0.2_tab5.0’ |
| | $c^{\mathsf{A}} = 0.3$ | ‘Ua0Ub3V0c0.3_tab5.0’ |
| | $c^{\mathsf{A}} = 0.4$ | ‘Ua0Ub3V0c0.4_tab5.0’ |
| | $c^{\mathsf{A}} = 0.5$ | ‘Ua0Ub3V0c0.5_tab5.0’ |
| **5** | $U = 2D,\ \underline{\mathrm{T}}^{\mathsf{AB}} = 0.2$ | ‘U2Va-1.5V1.5c0.5tab0.2’ |
| | $U = 2D,\ \underline{\mathrm{T}}^{\mathsf{AB}} = 1.0$ | ‘U2Va-1.5V1.5c0.5tab1.0’ |
| | $U = 2D,\ \underline{\mathrm{T}}^{\mathsf{AB}} = 3.0$ | ‘U2Va-1.5V1.5c0.5tab3.0’ |
| | $U = 4D,\ \underline{\mathrm{T}}^{\mathsf{AB}} = 0.2$ | ‘U4Va-1.5V1.5c0.5tab0.2’ |
| | $U = 4D,\ \underline{\mathrm{T}}^{\mathsf{AB}} = 1.0$ | ‘U4Va-1.5V1.5c0.5tab1.0’ |
| | $U = 4D,\ \underline{\mathrm{T}}^{\mathsf{AB}} = 3.0$ | ‘U4Va-1.5V1.5c0.5tab3.0’ |
| | $U = 6D,\ \underline{\mathrm{T}}^{\mathsf{AB}} = 0.2$ | ‘U6Va-1.5V1.5c0.5tab0.2’ |
| | $U = 6D,\ \underline{\mathrm{T}}^{\mathsf{AB}} = 1.0$ | ‘U6Va-1.5V1.5c0.5tab1.0’ |
| | $U = 6D,\ \underline{\mathrm{T}}^{\mathsf{AB}} = 3.0$ | ‘U6Va-1.5V1.5c0.5tab3.0’ |
